# Supplementary material for: Skyrmionic Transport and First Order Phase Transitions in Twisted Bilayer Graphene Quantum Hall Ferromagnet
Source: arXiv:2503.20392 source file (2025-10-09)
Supplement: Supplementary file 1 [file Supporting_Information.pdf]

**Supporting Information**

# Broken symmetry states and Quantum Hall Ferromagnetism in decoupled twisted bilayer graphene

Vineet Pandey,[†] Prasenjit Ghosh,[†] Riju Pal,[‡] Sourav Paul,[†] Abhijith M B,[†] Kenji Watanabe,[§] Takashi Taniguchi,[||] Atindra Nath Pal,[‡] and Vidya Kochat,[*,†]

[†]*Materials Science Centre, Indian Institute of Technology, Kharagpur, West Bengal – 721302, India*

[‡]*S. N. Bose National Centre for Basic Sciences, Kolkata, West Bengal- 700106, India.*

§*Research Center for Electronic and Optical Materials, National Institute for Materials Science, 1-1 Namiki, Tsukuba 305-0044, Japan*

[||]*Research Center for Materials Nanoarchitectonics, National Institute for Materials Science, 1-1 Namiki, Tsukuba 305-0044, Japan*

[*]E-mail: vidya@matsc.iitkgp.ac.in

## S1. Raman Spectroscopy of twisted bilayer graphene:

To characterize the twist angle (θ) of our devices, we employed Raman spectroscopy, a widely recognized technique for analyzing twisted bilayer graphene (TBLG). Previous Raman studies [1,2] have established that the R and R' modes, associated with LO phonons, exhibit a strong dependence on the twist angle.

Figure S1(a) presents the optical images of devices D1 and D2. The corresponding Raman maps highlight the overlap regions (dashed outlines) where two monolayer graphene layers form the TBLG system, as shown in Figure S1(b). The Raman spectra for devices D1 and D2 are displayed in Figure S1(c). For device D1, we observed the R' mode around 1625 $cm^{-1}$, which corresponds to a twist angle of approximately 5°, consistent with prior Raman studies on TBLG. Similarly, for device D2, the R mode was detected around 1426 $cm^{-1}$, indicating a twist angle of approximately 18°.

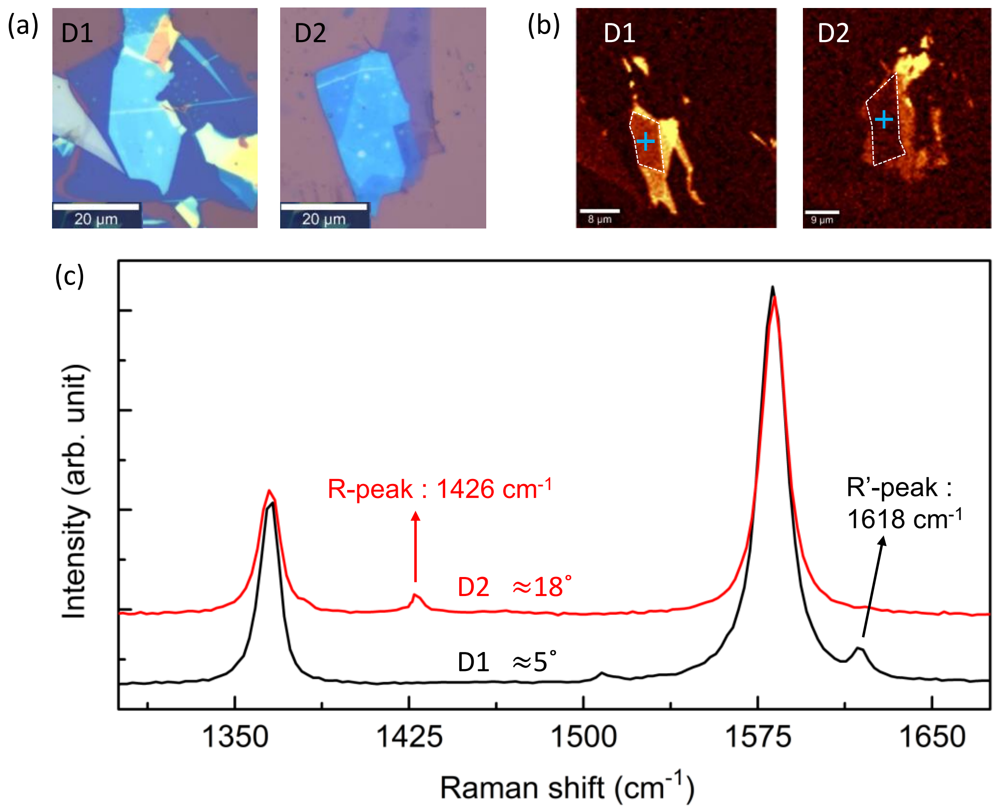


**Figure S1:** (a) Optical images of device D1 and D2. (b) Raman map of TBLG device samples. (c) Raman spectra of devices of D1 and D2.

**S2. Calculation of filling factors of upper ($\nu_U$) and lower ($\nu_L$) layers:**

To investigate how the upper ($n_U$) and lower ($n_L$) layer densities vary with $V_g$ in TBLG samples, we employ a model designed to calculate the layer densities in graphene double layers that are independently contacted and separated by a dielectric medium [3,4]. The applied back-gate voltage ($V_g$) is distributed between the $SiO_2$ dielectric and the Fermi energy of the lower graphene layer, described as:

$$e(V_g - V_D) = \frac{e^2(n_U + n_L)}{C_{BG}} + E_F(n_L) \ldots\ldots\ldots\ldots\ldots\ldots\ldots\ldots\ldots\ldots (1)$$

where, $V_D$ is the Dirac point offset and $C_{BG}$ is the back-gate capacitance of $SiO_2$ and h-BN. The Fermi energy relative to the charge neutrality point in monolayer graphene at a carrier density $n$ is given by $E_F(n) = sgn(n)\, \hbar v_f \sqrt{\pi|n|}$ , where $sgn(n)$ is signum function and determines the sign of $n$, and the Fermi velocity is given as $v_f$ ≈$10^8$ cm/s. The $E_F$ of the lower layer can be expressed as the sum of the electrostatic potential difference between the layers and the Fermi energy of the upper layer:

$$E_F(n_L) = \frac{e^2 n_U}{C_{int}} + E_F(n_U) \dots\dots\dots\dots\dots\dots\dots\dots\dots\dots\dots\dots\dots\dots.(2)$$

where $C_{int}$ is the interlayer capacitance between two layers of TBLG. For device D1, experimental $n_{U,L}$ *vs.* $V_g$ calculated using FFT analysis of SdH data (Figure 2(c)) in main text is linearly fitted with the equation (2), gives interlayer capacitance of $C_{int}$= (5.7±1) μF/cm as a fitting parameter, which agrees with the theoretically expected interlayer capacitance of Bernal-stacked bilayer graphene [5,6]. By using Eqs. (1) and (2) and using $C_{int} = 5.7$ μF/cm , we calculated $n_U$ and $n_L$ and the corresponding $n_{tot}(= n_U + n_L)$. The plot for $n_{U,L}$ vs $n_{tot}$ shown in Figure S2(a). The Fermi energy depends on both carrier density and magnetic field and is given by $E_F = E_N$ , where $E_N = sgn(N)v_f\sqrt{2e\hbar B|N|}$ is the energy of the $N^{\text{th}}$ Landau level (LL) in TBLG. Here, $N = Int\left[\frac{nh}{4eB}\right]$ represents the LL index, with $Int$ denoting the nearest integer function. Using $n_U$ and $n_L$ densities we calculated layer filling factors $v_{U,L} = \frac{n_{U,L}h}{eB}$. The plot $v_{U,L}$ vs $n_{tot}$ for 3T, 6T and 9T as shown in Figure S2(b). The black and red curve shown as $v_U$ and $v_L$ respectively in Figure 2(f) in the main text extracted from the calculated $v_{U,L}$ corresponding to B in steps of 0.5T and plotted as a function of $v_{tot}$.

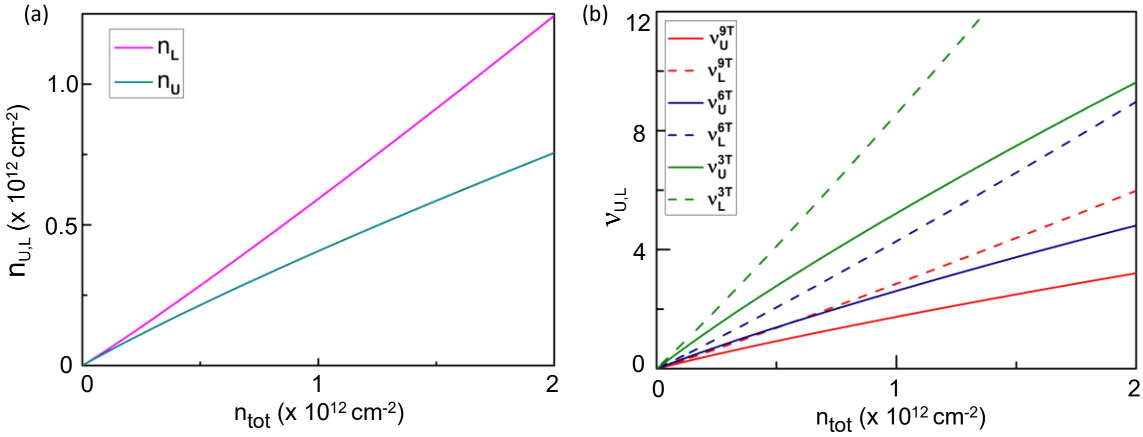


**Figure S2: (a)** Plot for calculated $n_{U,L}$ vs $n_{tot}$ for D1. **(b)** Plot calculated $v_{U,L}$ vs $n_{tot}$ at 3T, 6T and 9T for device D1.

**S3: Characterization of Device D2 to investigate Quantum Hall (QH) States and magnetoresistance: -**

Device D2 was characterized to explore the emergence of QH states and its magnetoresistance. Figure S3(a) illustrates the longitudinal resistance ($R_{xx}$) as a function of total carrier density ($n_{tot}$) at 300 K and 1.6 K in the absence of a magnetic field. The device exhibited low mobility (≈18,000 cm$^2$ V$^{-1}$ s$^{-1}$) Figure S3(b) presents $R_{xx}$ versus the total filling factor ($v_{tot}$) at 1.6 K under varying magnetic fields (B). Similar to Device D1, $R_{xx}$ increases at $v_{tot} = 0$ as B increases, but we do not observe a divergent behaviour till 9T. The broken symmetry QH states were also not observed in device D2 till 9T, due to lower mobility. Despite this low mobility and high disorder, QH states were observed at filling factors $v_{tot} = \pm 4, \pm 8, \pm 12, \pm 16 \dots$ similar to D1 (see main text), as shown in Figure S3(b).

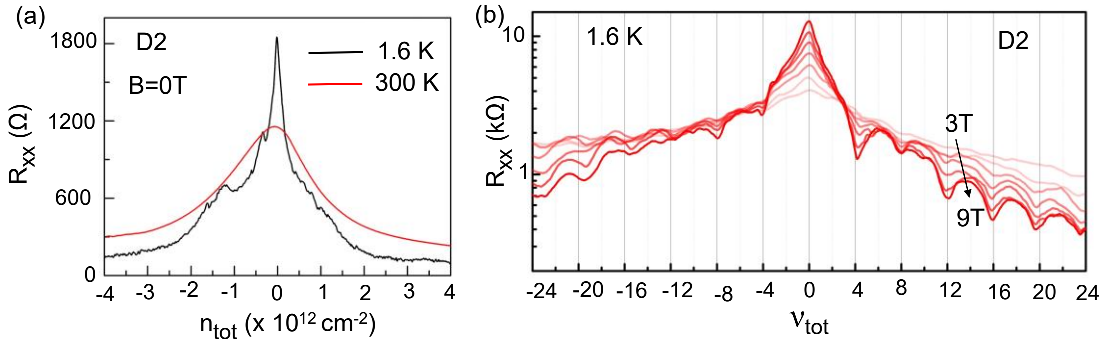


**Figure S3:** (a) Plot for $R_{xx}$ vs. $n_{tot}$ at 1.6 K and 300 K at 0T. (b) Plot for $R_{xx}$ vs. $\nu_{tot}$ shows QH states.

**S4: Temperature dependence of QH states and SdH oscillations for D1 and D2: -**

Figure S4(a)-(b) depicts the longitudinal resistance ($R_{xx}$) as a function of $\nu_{tot}$ at different temperatures for Device D1 and D2 respectively. At $\nu_{tot} = 0$, highly insulating behavior is observed at low temperatures. As the temperature increases, $R_{xx}$ at $\nu_{tot} = 0$ decreases due to the reduction of the QH insulator gap. The $R_{xx}$ minima at other integral filling factors and the SdH oscillations (in Figure S4(c)-(d)) vanish as temperature is increased due to the thermal broadening and carrier scattering effects when $k_B T \sim \Delta_{LL}$, where $\Delta_{LL}$ is the separation between the LLs.

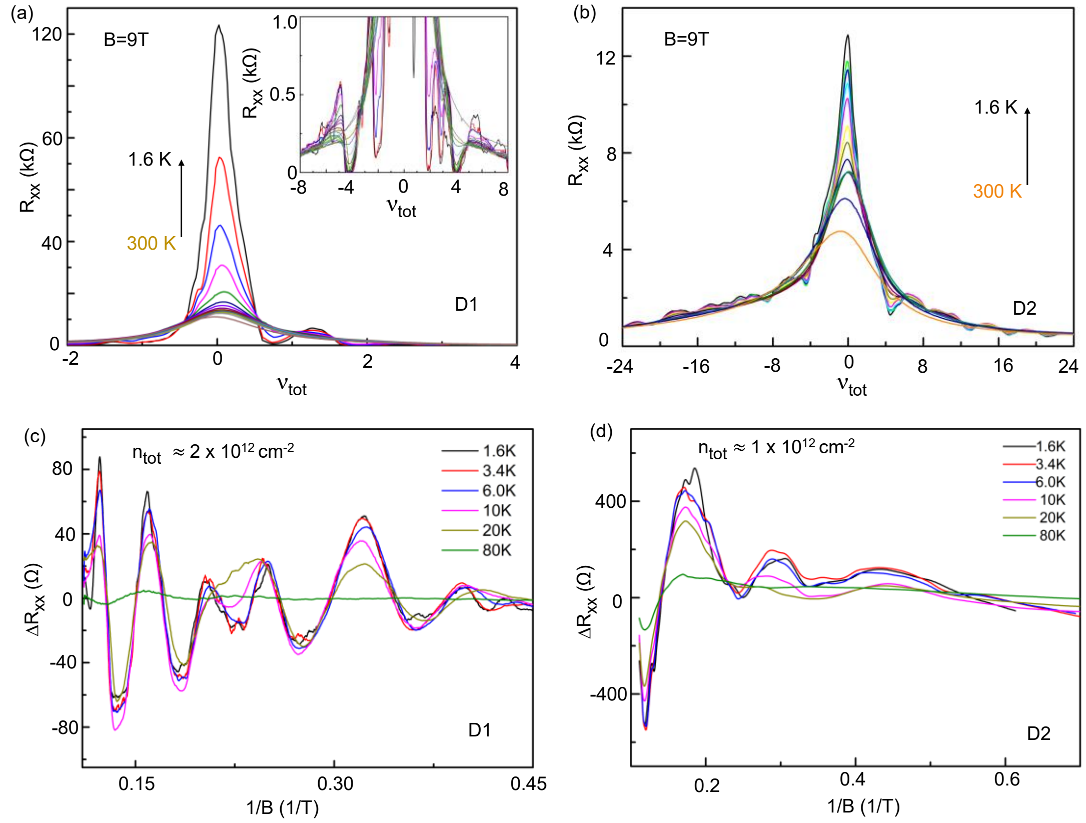


**Figure S4:** (a) Temperature dependence of $R_{xx}$ vs $\nu_{tot}$ near the CNP ($\nu_{tot} = 0$) for D1. (inset shows $R_{xx}$ vs $\nu_{tot}$ for higher $\nu_{tot}$values). (b) Temperature dependence of $R_{xx}$ vs $\nu_{tot}$ for D2. (c) and (d) shows temperature dependence of SdH oscillations for D1 and D2 respectively.

**S5: Magnetic field and temperature dependence of Dual sweep $R_{xx}$ for D2: -**

Figures S5(a) and S5(b) present the magnetic field (B) and temperature (T) dependence, respectively, of dual sweeps of $R_{xx}$ as a function of $\nu_{tot}$ for Device D2. Unlike Device D1, which exhibits significant hysteresis on both the electron and hole sides (as discussed in the main text), Device D2 shows negligible hysteresis over the range of B and T explored. In the B-dependence data shown in Figure S5(a), the emergence of QH states is observed with increasing magnetic field, consistent with the formation of Landau levels. However, the absence of notable hysteresis, in contrast to Device D1, suggests that hysteresis observed in D1 is most certainly due to the QH ferromagnetism arising from the broken symmetry states.

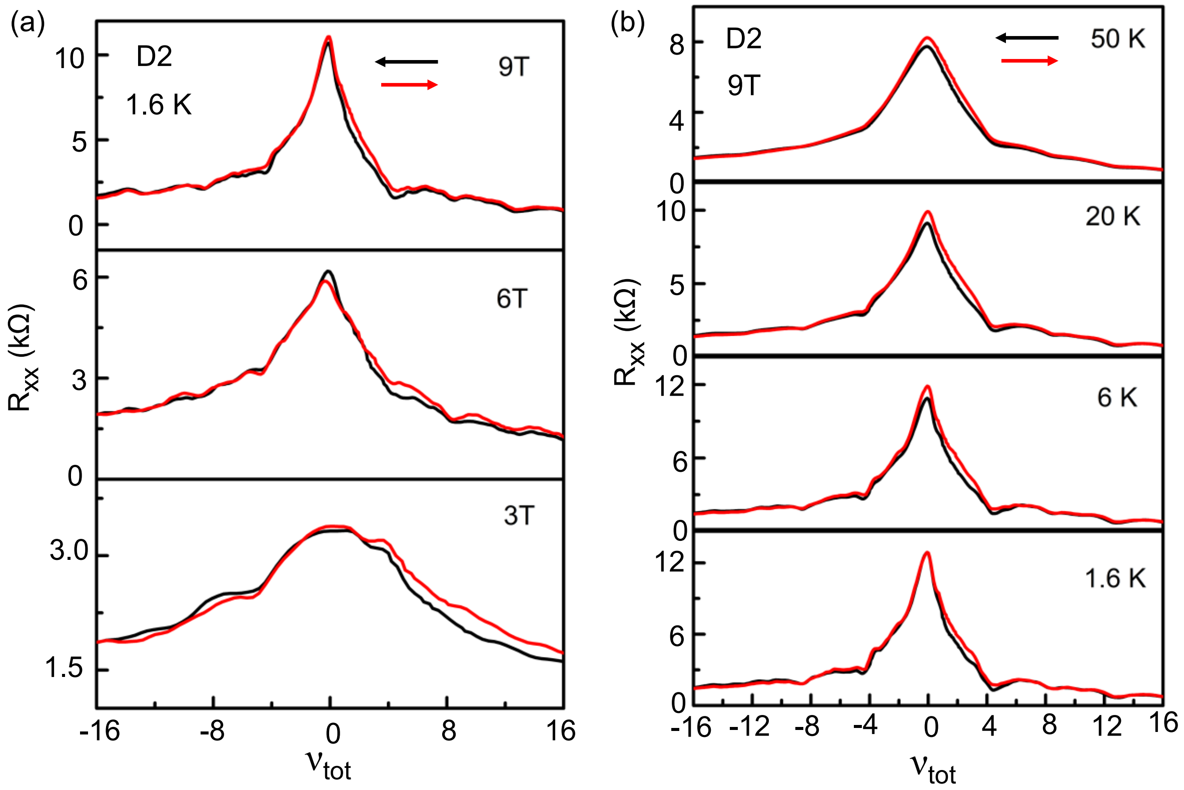


**Figure S5:** (a) Dual sweep $R_{xx}$ vs $\nu_{tot}$ for 3T, 6T and 9T. Black and Red arrow shows the direction of voltage sweep. (b)Temperature dependence of dual sweep $R_{xx}$ vs. $\nu_{tot}$ for 1.6K, 6K, 20K and 50K.

## References


1. Carozo, V.; Almeida, C. M.; Ferreira, E. H. M.; Cancado, L. G.; Achete, C. A.; Jorio, A. Raman Signature of Graphene Superlattices. *Nano Letters* **2011**, 11, 4527–4534.
2. Pandey, V.; Mishra, S.; Maity, N.; Paul, S.; B, A. M.; Roy, A. K.; Glavin, N. R.; Watanabe, K.; Taniguchi, T.; Singh, A. K.; Kochat, V. Probing Interlayer Interactions and Commensurate–Incommensurate Transition in Twisted Bilayer Graphene through Raman Spectroscopy. *ACS Nano* **2024**, 18, 4756–4764.

3. Fallahazad, B.; Hao, Y.; Lee, K.; Kim, S.; Ruoff, R. S.; Tutuc, E. Quantum Hall effect in Bernal stacked and twisted bilayer graphene grown on Cu by chemical vapor deposition. *Physical Review B* **2012**, 85, 201408.
4. Kim, S.; Jo, I.; Nah, J.; Yao, Z.; Banerjee, S. K.; Tutuc, E. Coulomb drag of massless fermions in graphene. *Physical Review B* **2011**, 83, 161401.
5. Min, H.; Sahu, B.; Banerjee, S. K.; MacDonald, A. H. Ab initio theory of gate induced gaps in graphene bilayers. *Physical Review B* **2007**, 75, 155115.
6. Schmidt, H.; Lüdtke, T.; Barthold, P.; McCann, E.; Fal'ko, V. I.; Haug, R. J. Tunable graphene system with two decoupled monolayers. *Applied Physics Letters* **2008**, 93.
